# Supplementary material for: Improving Crime Count Forecasts Using Twitter and Taxi Data
Source: arXiv:2009.03703 source file (2020-09-08)
Supplement: Supplementary file 1 [file appendix.tex]

The appendix provides some details related to estimation of the SAR, CAR and Poisson GLMM model and additional empirical results, which support the analysis in the main body of the paper. The latter include statistics for Moran's test of spatial correlation 
\section{Estimation details} \label{appendix}
This appendix details how the parameters of the SAR, CAR and Poisson GLMM model are estimated.% BLEH

Least-squares estimation of the parameters in the SAR model is inconsistent as the error is not independent. Instead, maximum likelihood estimates are obtained. The negative log likelihood can be minimised in stages where the maximum likelihood estimators for $\beta$ and $\sigma^2$ for fixed $\hat{\rho} W$ are as follows:
\begin{IEEEeqnarray}{rCl}
	\hat{\beta} & = & (X^\top X)^{{-1}}X^\top  (I_T \kron (I_N - \rho W))y \label{eq3:mlsarb}\\[0.2cm]
	\hat{\sigma}^2 & = & \frac{(y-(I_T\kron \rho W)y - X \hat{\beta})^\top}{\raisebox{-1pt}{$NT$}} \nonumber \\
	&&\frac{(y-(I_T\kron \rho W)y - X \hat{\beta})}{\raisebox{-1pt}{$NT$}} \label{eq3:mlsarv}.
\end{IEEEeqnarray}
Substituting the estimators in (\ref{eq3:mlsarb}) and (\ref{eq3:mlsarv}) back into the likelihood to obtain the maximum likelihood estimate of $\rho B$ yields a negative log likelihood depending only on $\rho$:
\begin{IEEEeqnarray}{rCl}
	\log \mathcal{L} &=& -\log \vert I_T \kron (I_N - \rho W) \vert + \frac{NT}{2} \log2\pi \nonumber \\[0.15cm]
	&&+\> \frac{NT}{2} \log \frac{(e_0 - \rho e_L)^\top(e_0 - \rho e_L)}{\raisebox{-1pt}{$NT$}} \label{eq4:conclogsar},
\end{IEEEeqnarray}
where $\vert \cdot \vert$ denotes the determinant and where $e_0$ and $e_L$ of regressing $y$ on $X$ and $Wy$ on $X$, respectively \citep[see][p.~256]{anselin1998spatial}.
The parameter space of $\rho$ is restricted to $1/\omega_{\rm min} \leq \rho \leq 1/\omega_{\rm max}$ where $\omega$ denotes the eigenvalues of matrix $W$ to ensure positive definiteness of $I_N - \rho W$ \citep[p.~381]{elhorst2010spatial}.

As in the SAR model, the CAR parameters are estimated by minimising the negative log likelihood in stages by alternating between estimation of $\beta$ and $\sigma^2$ with $\hat{\delta} W$ fixed. The $\beta$ and $\sigma$ estimates are given by:
\begin{IEEEeqnarray}{rCl}
	\hat{\beta} &=& (X^\top BX)^{{-1}}X^\top By \label{eq4:mlcarb}\\[0.2cm]
	\hat{\sigma}^2 &=& \frac{\hat{\varepsilon}^\top B \hat{\varepsilon}}{\raisebox{-1pt}{$NT$}}, \label{eq4:mlcarv}
\end{IEEEeqnarray}
where $B$ is $\left(I_T \kron (I_N - \delta W)\right)$. These estimates are plugged into the log likelihood which gives the following negative log likelihood depending on $\delta$ only  \citep[p.~467]{cressie1993statistics}:
\begin{IEEEeqnarray}{rCl} 
	\log \mathcal{L} & =& -\frac{1}{2} \log \vert B \vert + \frac{NT}{2} \log2\pi \nonumber \\[0.15cm]
	&&+\> \frac{NT}{2} \log \frac{\hat{\varepsilon}^\top B \hat{\varepsilon}}{\raisebox{-1pt}{$NT$}}.
\end{IEEEeqnarray}
During optimisation, the parameter space for $\hat{\delta}$ needs to be restricted, too, to the inverse of the smallest and largest eigenvalues of $W$ to ensure positive definiteness of $I_N - \delta W$. 

In REML, the dependent data is first transformed by substracting the fixed effects and then used to obtain estimates of the regression coefficients $\beta$ and $\eta$ via iteratively reweighted least squares. The variance parameter $\sigma^2$ can then be estimated by maximising the restricted log likelihood holding the regression estimators constant. Both estimation procedures are alternated until the estimators converge. Details are given in \citet{kneibrestricted}.

\section{Analysis of Spatial Correlation} \label{{app.Spatial}}
As indicated in the main part of the paper, we check the strength of spatial correlation between areal units using Moran's $I$ \citep[p.~75]{banerjee2015hierarchical}. Note that with panel data, spatial dependence is only tested within cross-sections, i.e. within the same time period $t$ \citep[p.~627]{anselin2008spatial}. Table~\ref{tbla:moran} reports the results of testing the cross-sectional observations $y_t$ with all variables for each period on violent and property crime data. Table~\ref{tbla:moran} clearly shows that the crime counts are spatially dependent. For the property crime data, we obtain an average Moran's $I$ value of 0.2565, which provides strong evidence against the null hypothesis of no spatial correlation. The average Moran's $I$ value for the violent crime data is 0.1446, which also facilitates rejecting the null hypothesis with high confidence. 

\begin{table}[ht]
	\centering
	\begin{tabular}{crrrr}
		\toprule
		& \multicolumn{2}{c}{Property Counts} & \multicolumn{2}{c}{Violent Counts} \\ \cmidrule{2-5}
		Week & \multicolumn{1}{c}{$I$} & \multicolumn{1}{c}{$p$} & \multicolumn{1}{c}{$I$} & \multicolumn{1}{c}{$p$}\\ 
		\midrule
		23 & 0.2459 & 0.0000 & 0.1118 & 0.0000 \\ 
		24 & 0.2679 & 0.0000 & 0.1481 & 0.0000 \\ 
		25 & 0.2087 & 0.0000 & 0.1052 & 0.0000 \\ 
		26 & 0.2721 & 0.0000 & 0.0988 & 0.0000 \\ 
		27 & 0.2517 & 0.0000 & 0.1290 & 0.0000 \\ 
		28 & 0.2444 & 0.0000 & 0.1690 & 0.0000 \\ 
		29 & 0.2593 & 0.0000 & 0.1725 & 0.0000 \\ 
		30 & 0.2584 & 0.0000 & 0.1834 & 0.0000 \\ 
		31 & 0.3014 & 0.0000 & 0.1737 & 0.0000 \\ 
		32 & 0.2494 & 0.0000 & 0.1673 & 0.0000 \\ 
		33 & 0.2279 & 0.0000 & 0.1894 & 0.0000 \\ 
		34 & 0.2537 & 0.0000 & 0.1636 & 0.0000 \\ 
		35 & 0.3048 & 0.0000 & 0.1252 & 0.0000 \\ 
		36 & 0.2911 & 0.0000 & 0.1179 & 0.0000 \\ 
		37 & 0.2517 & 0.0000 & 0.1632 & 0.0000 \\ 
		38 & 0.2960 & 0.0000 & 0.1723 & 0.0000 \\ 
		39 & 0.2482 & 0.0000 & 0.1358 & 0.0000 \\ 
		40 & 0.2504 & 0.0000 & 0.1448 & 0.0000 \\ 
		41 & 0.2840 & 0.0000 & 0.1485 & 0.0000 \\ 
		42 & 0.2517 & 0.0000 & 0.1375 & 0.0000 \\ 
		43 & 0.2519 & 0.0000 & 0.1444 & 0.0000 \\ 
		44 & 0.2461 & 0.0000 & 0.1504 & 0.0000 \\ 
		45 & 0.2538 & 0.0000 & 0.1244 & 0.0000 \\ 
		46 & 0.2564 & 0.0000 & 0.0946 & 0.0000 \\ 
		47 & 0.2327 & 0.0000 & 0.1490 & 0.0000 \\ 
		48 & 0.2100 & 0.0000 & 0.1393 & 0.0000 \\ 
		\bottomrule
	\end{tabular}
\caption[Estimated Moran's $I$ statistics]{Estimated Moran's $I$ statistics and $z$-values for crime counts based on 26 weeks of data and $N$ = 1974 spatial units.}
\label{tbla:moran}
\end{table}

A further test for spatial dependence is the test proposed by \citet{singh1983test}, which is performed on the residuals $e = y - X\hat{\beta}_{OLS}$. For details see \citet[p.~524]{singh1983test}. For both crime types, the null hypothesis of no spatial dependence, is rejected with $p$-values of 0.0000.

\section{Analysis of Correlation Across Violence and Property Crime}
\todoin{need some brief description if we keep the table}

\begin{table}
	\centering
\begin{tabular}{l*{2}{S[table-format=-1.2]}} \toprule
	Variable & {Property} & {Violent} \\ \midrule
	Violent Crime & 0.17 & 1.00\\
	Population & 0.20 & 0.19 \\
	Age & -0.05 & -0.17\\
	Male & 0.05 & -0.05 \\
	Black & -0.03 & 0.16 \\
	Asian & -0.02 & -0.13 \\ 
	Hispanic & 0.03 & 0.21 \\
	Vacancy & 0.17 & -0.02 \\
	Female-headed HH & -0.06 & 0.27 \\
	Log night tweets & 0.41 & 0.09 \\
	Taxi$^1$ & 0.48 & 0.44 \\ \bottomrule
	\multicolumn{3}{l}{\footnotesize{$^1$Lagged by the specific crime type}}\\ 
\end{tabular}
\caption{Correlation matrix}
\label{tbl:correlationtable}
\end{table}
